# Supplementary material for: Real-Time Distributed Model Predictive Control with Limited Communication Data Rates
Source: arXiv:2208.12531 source file (2023-08-05)
Supplement: Supplementary file 1 [file appendix.tex]

\subsection{Lemma 1 proof}
\begin{proof}
Constraint \eqref{sufficient condition 1} and \eqref{sufficient condition 2} can be written as 
\begin{subequations}
\begin{align}
    & Y_1 [ C_\alpha , C_\beta ] ^\top \geq \bar{\rho}_0, \label{hyperplane 1}\\
  &  Y_2 [ C_\alpha , C_\beta ] ^\top \geq \bar{\rho}_0, \label{hyperplane 2}
\end{align}
\end{subequations}
where $Y_1 = [\frac{2^n-a_2}{2^{n+1} a_1}, -\frac{a_3}{2^{n+1} a_1}]$ and $Y_2 = [-\frac{b_3}{2^{n+1} b_1}, \frac{2^n-b_2}{2^{n+1} b_1} ]$. As shown in Fig. \ref{intersection}, $Y_1$ and $Y_2$ define two hyperplanes $\mathcal{H}_1$ and $\mathcal{H}_2$, respectively, in the plane spanned by $C_\alpha$ and $C_\beta$.

Since $\frac{a_3}{2^{n+1} a_1}, \frac{b_3}{2^{n+1} b_1},\bar{\rho}_0 > 0$, $\mathcal{H}_1$ intersects the positive $C_\alpha$-axis and $\mathcal{H}_2$ intersects the positive $C_\beta$-axis.
Meanwhile, value of $\frac{2^n-a_2}{2^{n+1} a_1}$ and $\frac{2^n-b_2}{2^{n+1} b_1}$ depend on $n$, affecting slopes and point of intersection of $\mathcal{H}_1$ and $\mathcal{H}_2$.
Fig. \ref{intersection} shows that \eqref{sufficient condition 3} is satisfied only when both $\mathcal{H}_1$ and $\mathcal{H}_2$ have positive slopes, which can be guaranteed if
\begin{align}
    & 2^{n}-b_2 > 0, \:\: 2^{n}-a_2 > 0, \label{positive slope condition } 
\end{align}
and intersect each other in the positive orthant, which can be guaranteed if
\begin{align}
    & \frac{2^{n}-b_2}{b_3} > \frac{a_3}{2^{n}-a_2}. \label{intersection condition}
\end{align}
\eqref{intersection condition} can be rewritten as
\begin{equation}
    (2^n)^2 - (a_2+b_2) 2^n + (a_2 b_2 - a_3 b_3) > 0.
\end{equation}
According to the quadratic formula, the l.h.s. intersects the $2^n$-axis at ${0.5 (a_2+  b_2 \pm \sqrt{a_2^2 +b_2^2 - 2 a_2 b_2 + 4 a_3 b_3})}$. 
It is easy to see if $a_2^2 +b_2^2 - 2 a_2 b_2 + 4 a_3 b_3 \leq 0$, \eqref{intersection condition} is automatically satisfied.
If $a_2^2 +b_2^2 - 2 a_2 b_2 + 4 a_3 b_3 > 0$, \eqref{intersection condition} is satisfied if $2^n < {0.5(a_2+b_2 + \sqrt{a_2^2 +b_2^2 - 2 a_2 b_2 + 4 a_3 b_3})}$ and $2^n > {0.5(a_2+b_2 + \sqrt{a_2^2 +b_2^2 - 2 a_2 b_2 + 4 a_3 b_3})}$. If \eqref{positive slope condition } holds, only the second inequality needs to be considered. 
Thus, to satisfy \eqref{intersection condition} is to have 
\begin{equation} \label{n third condition}
    2^n >  {0.5(a_2+b_2 + \operatorname{Re}(\sqrt{a_2^2 +b_2^2 - 2 a_2 b_2 + 4 a_3 b_3}))}.
\end{equation}
Finally, taking $\operatorname{log_2}$ on both sides of \eqref{positive slope condition } and \eqref{n third condition} and combining them gives the claim.
\end{proof}
